# Supplementary material for: Variational Calibration of Computer Models
Source: arXiv:1810.12177 source file (2018-10-29)
Supplement: Supplementary file 1 [file supplement.tex]

\documentclass{article}

\setlength{\textheight}{22cm}
\setlength{\topmargin}{-1.2cm}
\addtolength{\oddsidemargin}{-60pt}
\addtolength{\textwidth}{120pt}

%\usepackage{aistats2019}
% If your paper is accepted, change the options for the package
% aistats2019 as follows:
%
%% \usepackage{aistats2019_singlecol}
%
% This option will print headings for the title of your paper and
% headings for the authors names, plus a copyright note at the end of
% the first column of the first page.

% If you set papersize explicitly, activate the following three lines:
%\special{papersize = 8.5in, 11in}
%\setlength{\pdfpageheight}{11in}
%\setlength{\pdfpagewidth}{8.5in}

% If you use natbib package, activate the following three lines:
\usepackage[round]{natbib}

% If you use BibTeX in apalike style, activate the following line:
%% \bibliographystyle{apalike}

%%%%%%%%%%%%%%% personnal shortcut and packages
\usepackage {tikz}  % for tikz figures
\usetikzlibrary {positioning}
\usetikzlibrary{fit}
\usetikzlibrary{backgrounds}
\usepackage{amssymb}% for \mathbb (board bold)
\usepackage{amsmath}

\usepackage{xspace}

\input{notation.tex}

% setting of the latex figures (\ref{fig:concept} and \ref{fig:nn})
\definecolor {processblue}{cmyk}{0.2,.1,0.1,.0}
\definecolor {randomblue}{cmyk}{0.57,0.05,0,0.76}
\definecolor {lightleafyellow}{cmyk}{.00,.29,.67,.68}
\definecolor {leafyellow}{cmyk}{.00,.30,.98,.30}
\definecolor {treeorange}{cmyk}{.00,.67,.83,.09}
\definecolor {grassgreen}{cmyk}{.99,.0,.23,.40}
\newdimen\microwidth 
\newdimen\microheight
\newdimen\circlediameter
\microwidth  = 0.045\linewidth
\microheight = 0.065\linewidth
\circlediameter = 0 cm
\newdimen\microwidthB 
\newdimen\microheightB
\newdimen\circlediameterB
\microwidthB  = 0.06\linewidth
\microheightB = 0.06\linewidth
\circlediameterB = 0 cm

\title{Supplementary Material for the Paper: \\Variational Calibration of Computer Models}

\date{}

\begin{document}

\maketitle

\input{appendix}

%% \bibliography{biblio}
%% \bibliographystyle{abbrvnat_nourl}
%\bibliographystyle{abbrv}
%\bibliographystyle{apalike}
\end{document}
